# Supplementary material for: WoundAIssist: Development and Evaluation of an AI-Based Mobile Application for Remote Chronic Wound Care in Elderly Patients
Source: arXiv:2506.06104 source file (2026-09-17)
Supplement: Supplementary file 1 [file 10-appendix.tex]

\section{Screenshots of the Low-Fidelity Prototype}
\label{appendix:screenshots_low_fidelity}

For completeness, we include screenshots of our digital low-fidelity prototype used in the initial usability study in Figure~\ref{fig:appendix:low_fidelity:screenshots_app}. We focus on the functionalities that have changed the most, omitting some of the screens that did not change in the transition from low-fidelity to high-fidelity prototype (e.g., overview, questionnaires, video chat). 
%, such as the patient overview, the two questionnaire screens, or the video chat function.
\begin{figure*}[ht!]
    \centering
    \begin{subfigure}{0.23\textwidth}
        \centering
        \includegraphics[width=\linewidth]{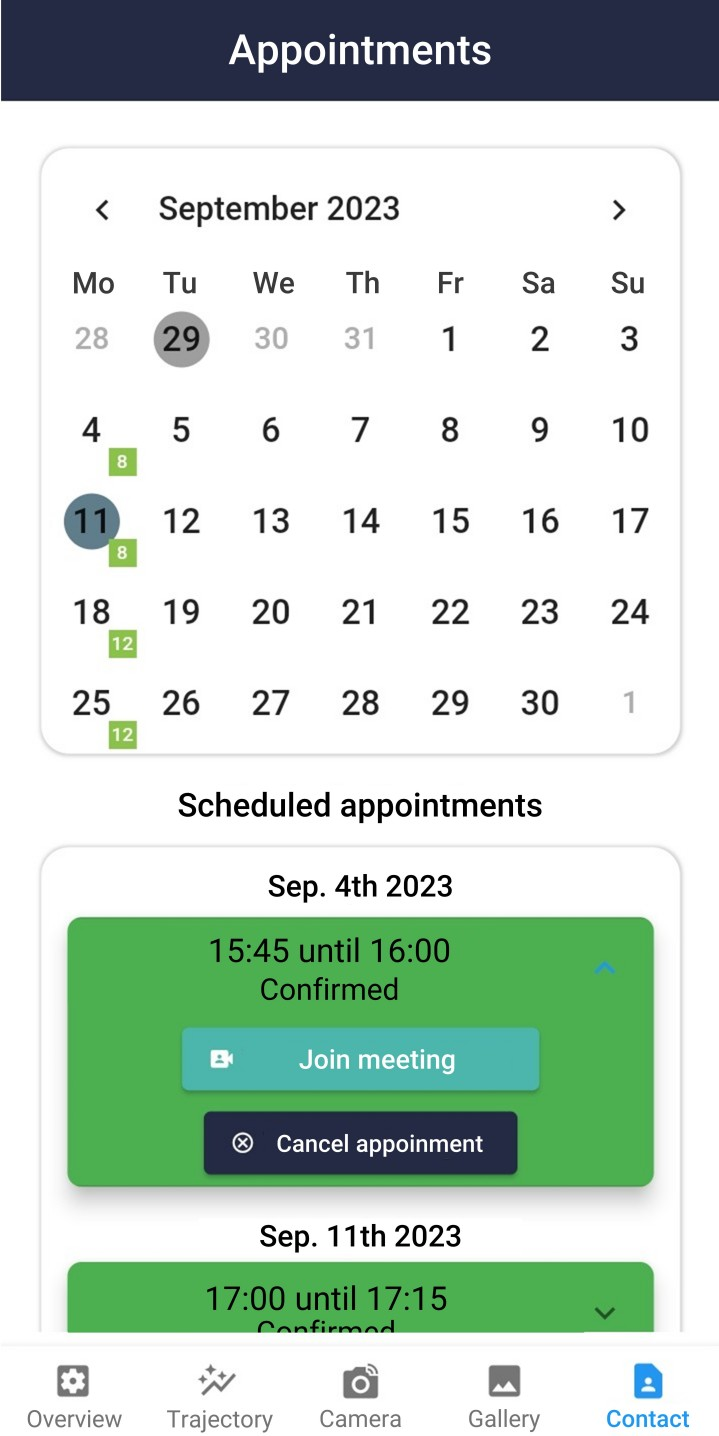}
        \caption{Calendar \textit{(misnamed)}}
        \label{fig:appendix:low_fidelity:calendar}
    \end{subfigure} \hfill
    \begin{subfigure}{0.23\textwidth}
        \centering
        \includegraphics[width=\linewidth]{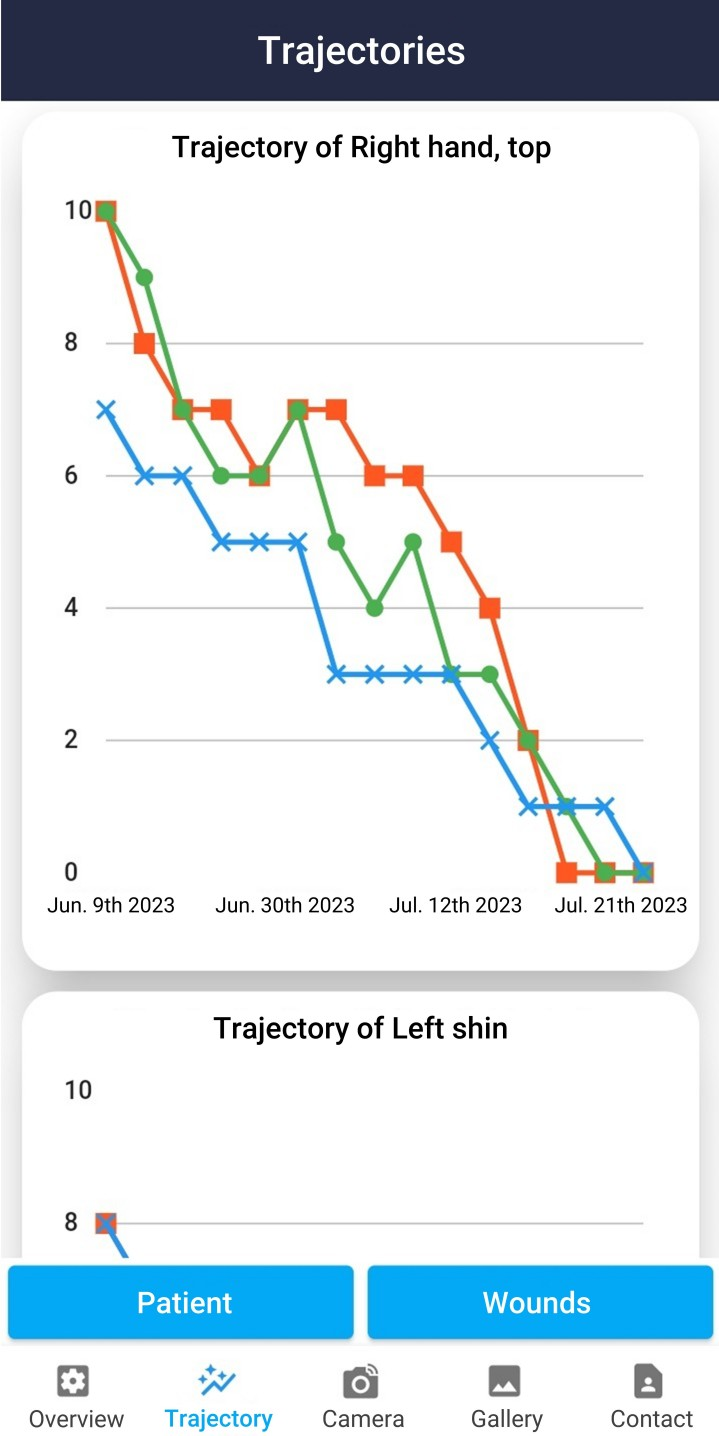}
        \caption{Wound trajectory}
        \label{fig:appendix:low_fidelity:wound_trajectory}
    \end{subfigure} \hfill
    \begin{subfigure}{0.23\textwidth}
        \centering
        \includegraphics[width=\linewidth]{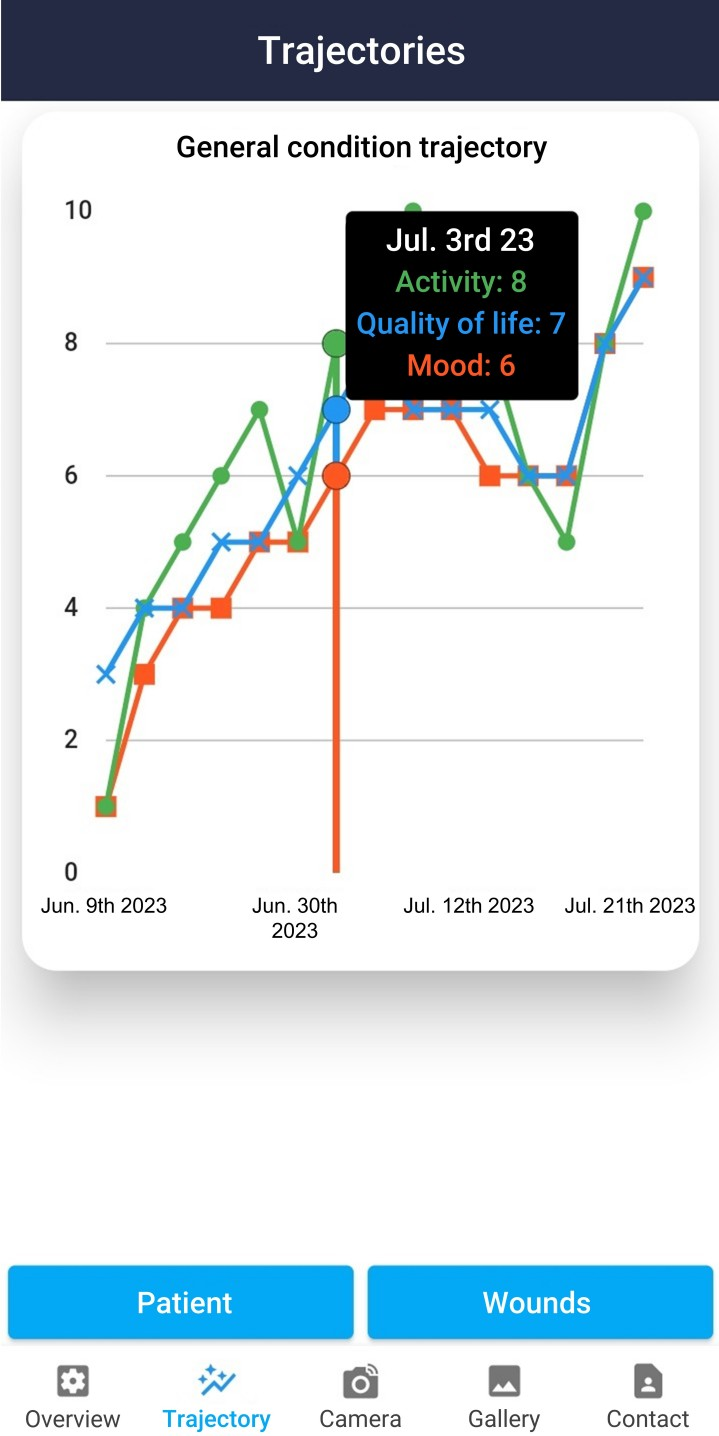}
        \caption{General health trajectory}
        \label{fig:appendix:low_fidelity:general_condition_trajectory}
    \end{subfigure} \hfill   
    \begin{subfigure}{0.23\textwidth}
        \centering
        \includegraphics[width=\linewidth]{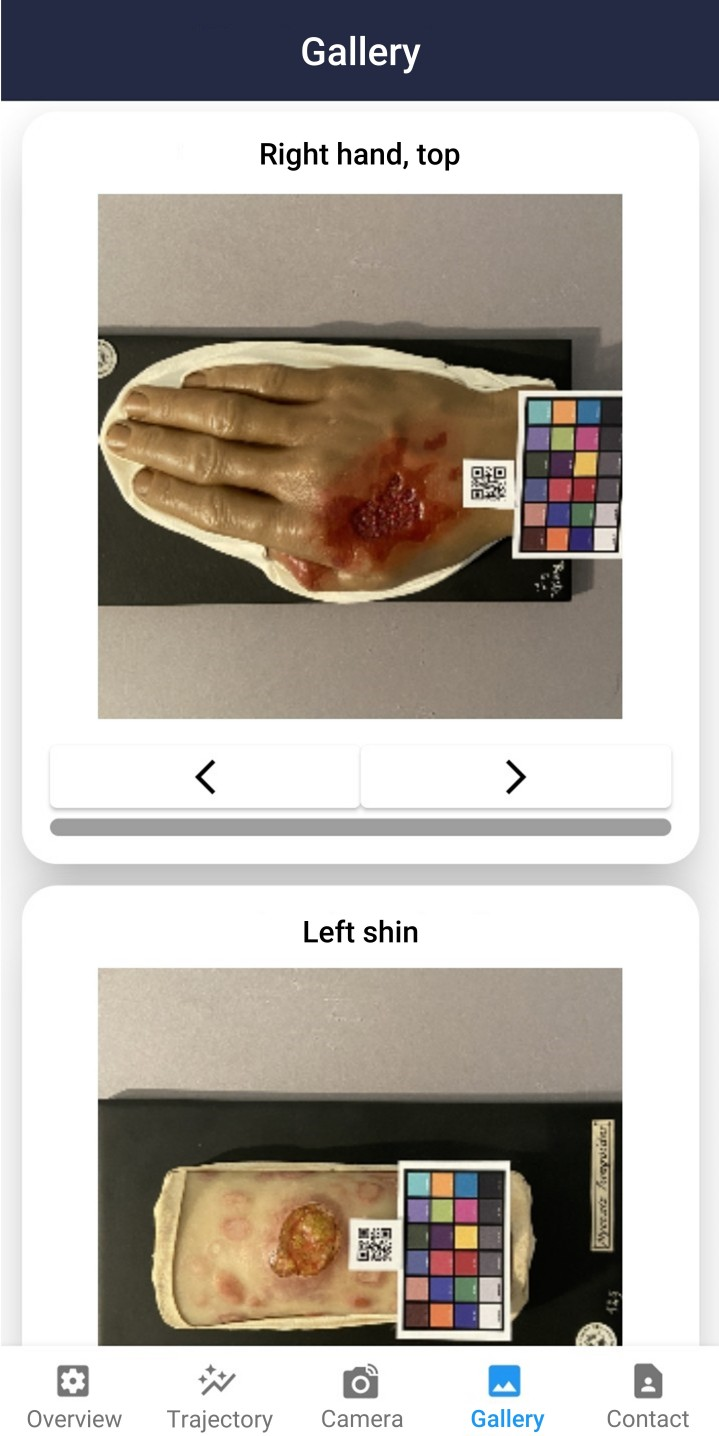}
        \caption{Gallery \textit{(w/o counter)}}
        \label{fig:appendix:low_fidelity:gallery}
    \end{subfigure} \hfill
    \\\vspace{0.5cm} % Adds vertical space between rows
    \begin{subfigure}{0.3\textwidth}
        \centering
        \includegraphics[width=0.76\linewidth]{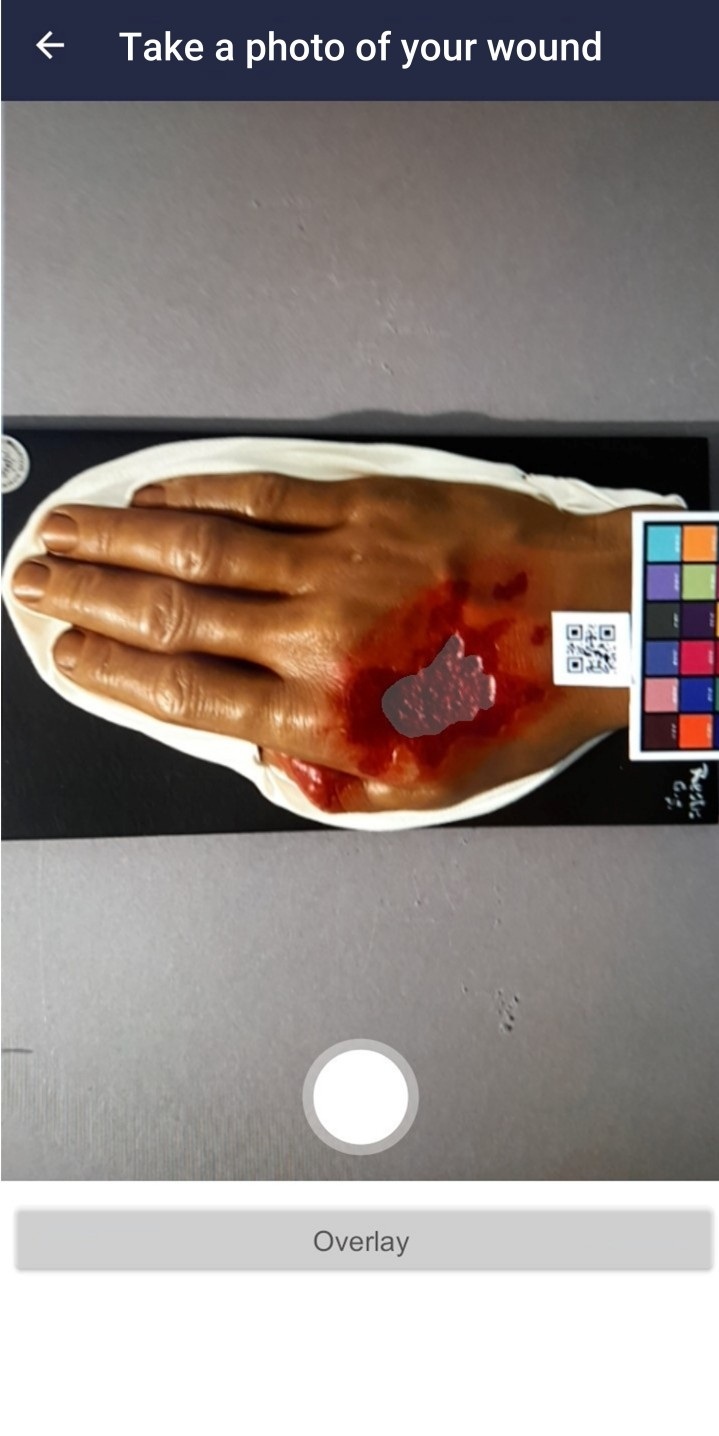}
        \caption{Camera screen with overlay}
        \label{fig:appendix:low_fidelity:camera_screen}
    \end{subfigure} \hfill
        \begin{subfigure}{0.3\textwidth}
        \centering
        \includegraphics[width=0.76\linewidth]{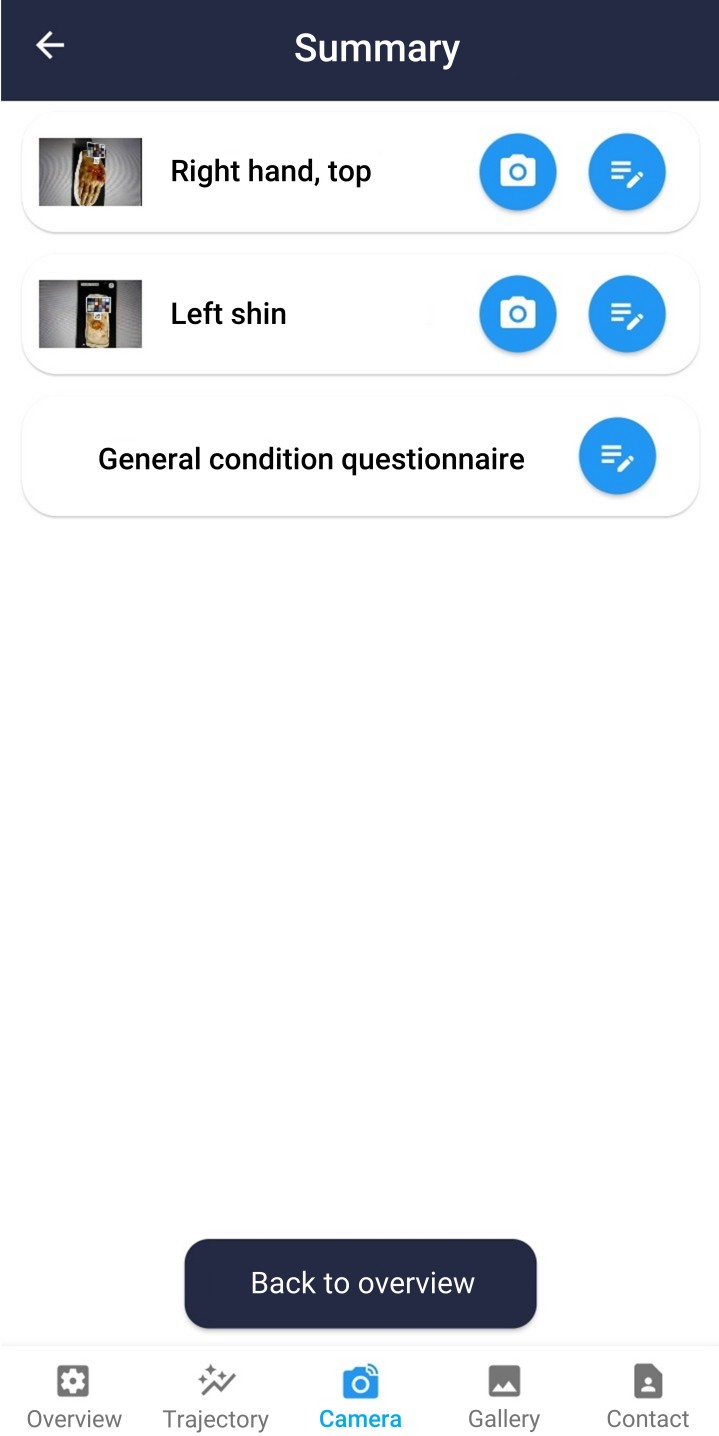}
        \caption{Summary \textit{(w/o help icon)}}
        \label{fig:appendix:low_fidelity:summary_view}
    \end{subfigure} \hfill
    \begin{subfigure}{0.3\textwidth}
        \centering
        \includegraphics[width=0.76\linewidth]{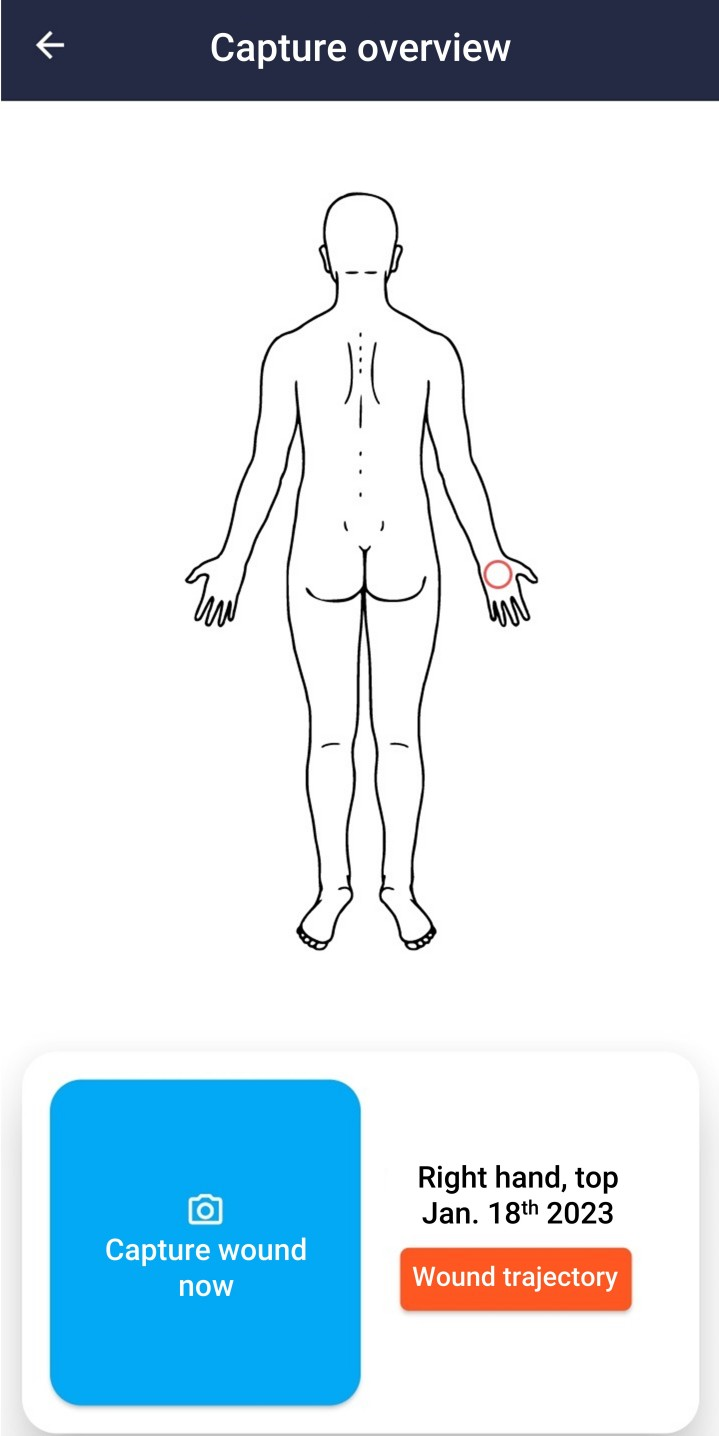}
        \caption{Wound localization (back)}
        \label{fig:appendix:low_fidelity:wound_localization}
    \end{subfigure} 
    \caption{Excerpt of screenshots of our low-fidelity prototype.}
    \label{fig:appendix:low_fidelity:screenshots_app}
    \Description{Seven app screenshots, displaying the functionalities of the low-fidelity prototype that were changed the most: The calendar function with confirmed appointments; separate trajectories for wound-specific parameters and overall condition; the image gallery with previews of captured images, the previous camera interface with an overlay during image capture, the summary view shown after completing documentation, and the wound localization feature highlighting a wound on the back of the body.}
\end{figure*}
